# Supplementary material for: Metric and arithmetic properties of mediant-Rosen maps
Source: arXiv:0812.0548 source file (2008-12-02)
Supplement: Supplementary file 1 [file supp-pdf.tex]

\endinput
